# Supplementary material for: Structural Estimation of Partially Observable Markov Decision Processes
Source: arXiv:2008.00500 source file (2021-12-28)
Supplement: Supplementary file 1 [file appendix.tex]

This is the appendix
